# Supplementary material for: Deterministic Non-cooperative Binding in Two-Dimensional Tile Assembly Systems Must Have Ultimately Periodic Paths
Source: arXiv:2202.05165 source file (2022-02-09)
Supplement: Supplementary file 1 [file appendices.tex]

\clearpage
\appendix

%%%%%%%%%%%%%%%%%%%%%%%%%%%%%%
%%%%%%%%%%%%%%%%%%%%%%%%%%%%%%
%\section*{The Rest is for Reviewing Only}
%%%%%%%%%%%%%%%%%%%%%%%%%%%%%%
%%%%%%%%%%%%%%%%%%%%%%%%%%%%%%

%\tableofcontents

\JDLvocabularyTableofsymbols

% ;;; Local Variables: ***
% ;;; eval: (flyspell-mode) ***
% ;;; eval: (ispell-change-dictionary "british" nil) ***
% ;;; eval: (flyspell-buffer) ***
% ;;; End: ***
